# Supplementary material for: Difference-in-Differences with Multiple Events
Source: arXiv:2409.05184 source file (2025-01-21)
Supplement: Supplementary file 1 [file 99-appendix.tex]

\begin{frame}[label=app]{Appendix}

\begin{figure}
    \centering
    \includegraphics[width=0.6\textwidth]{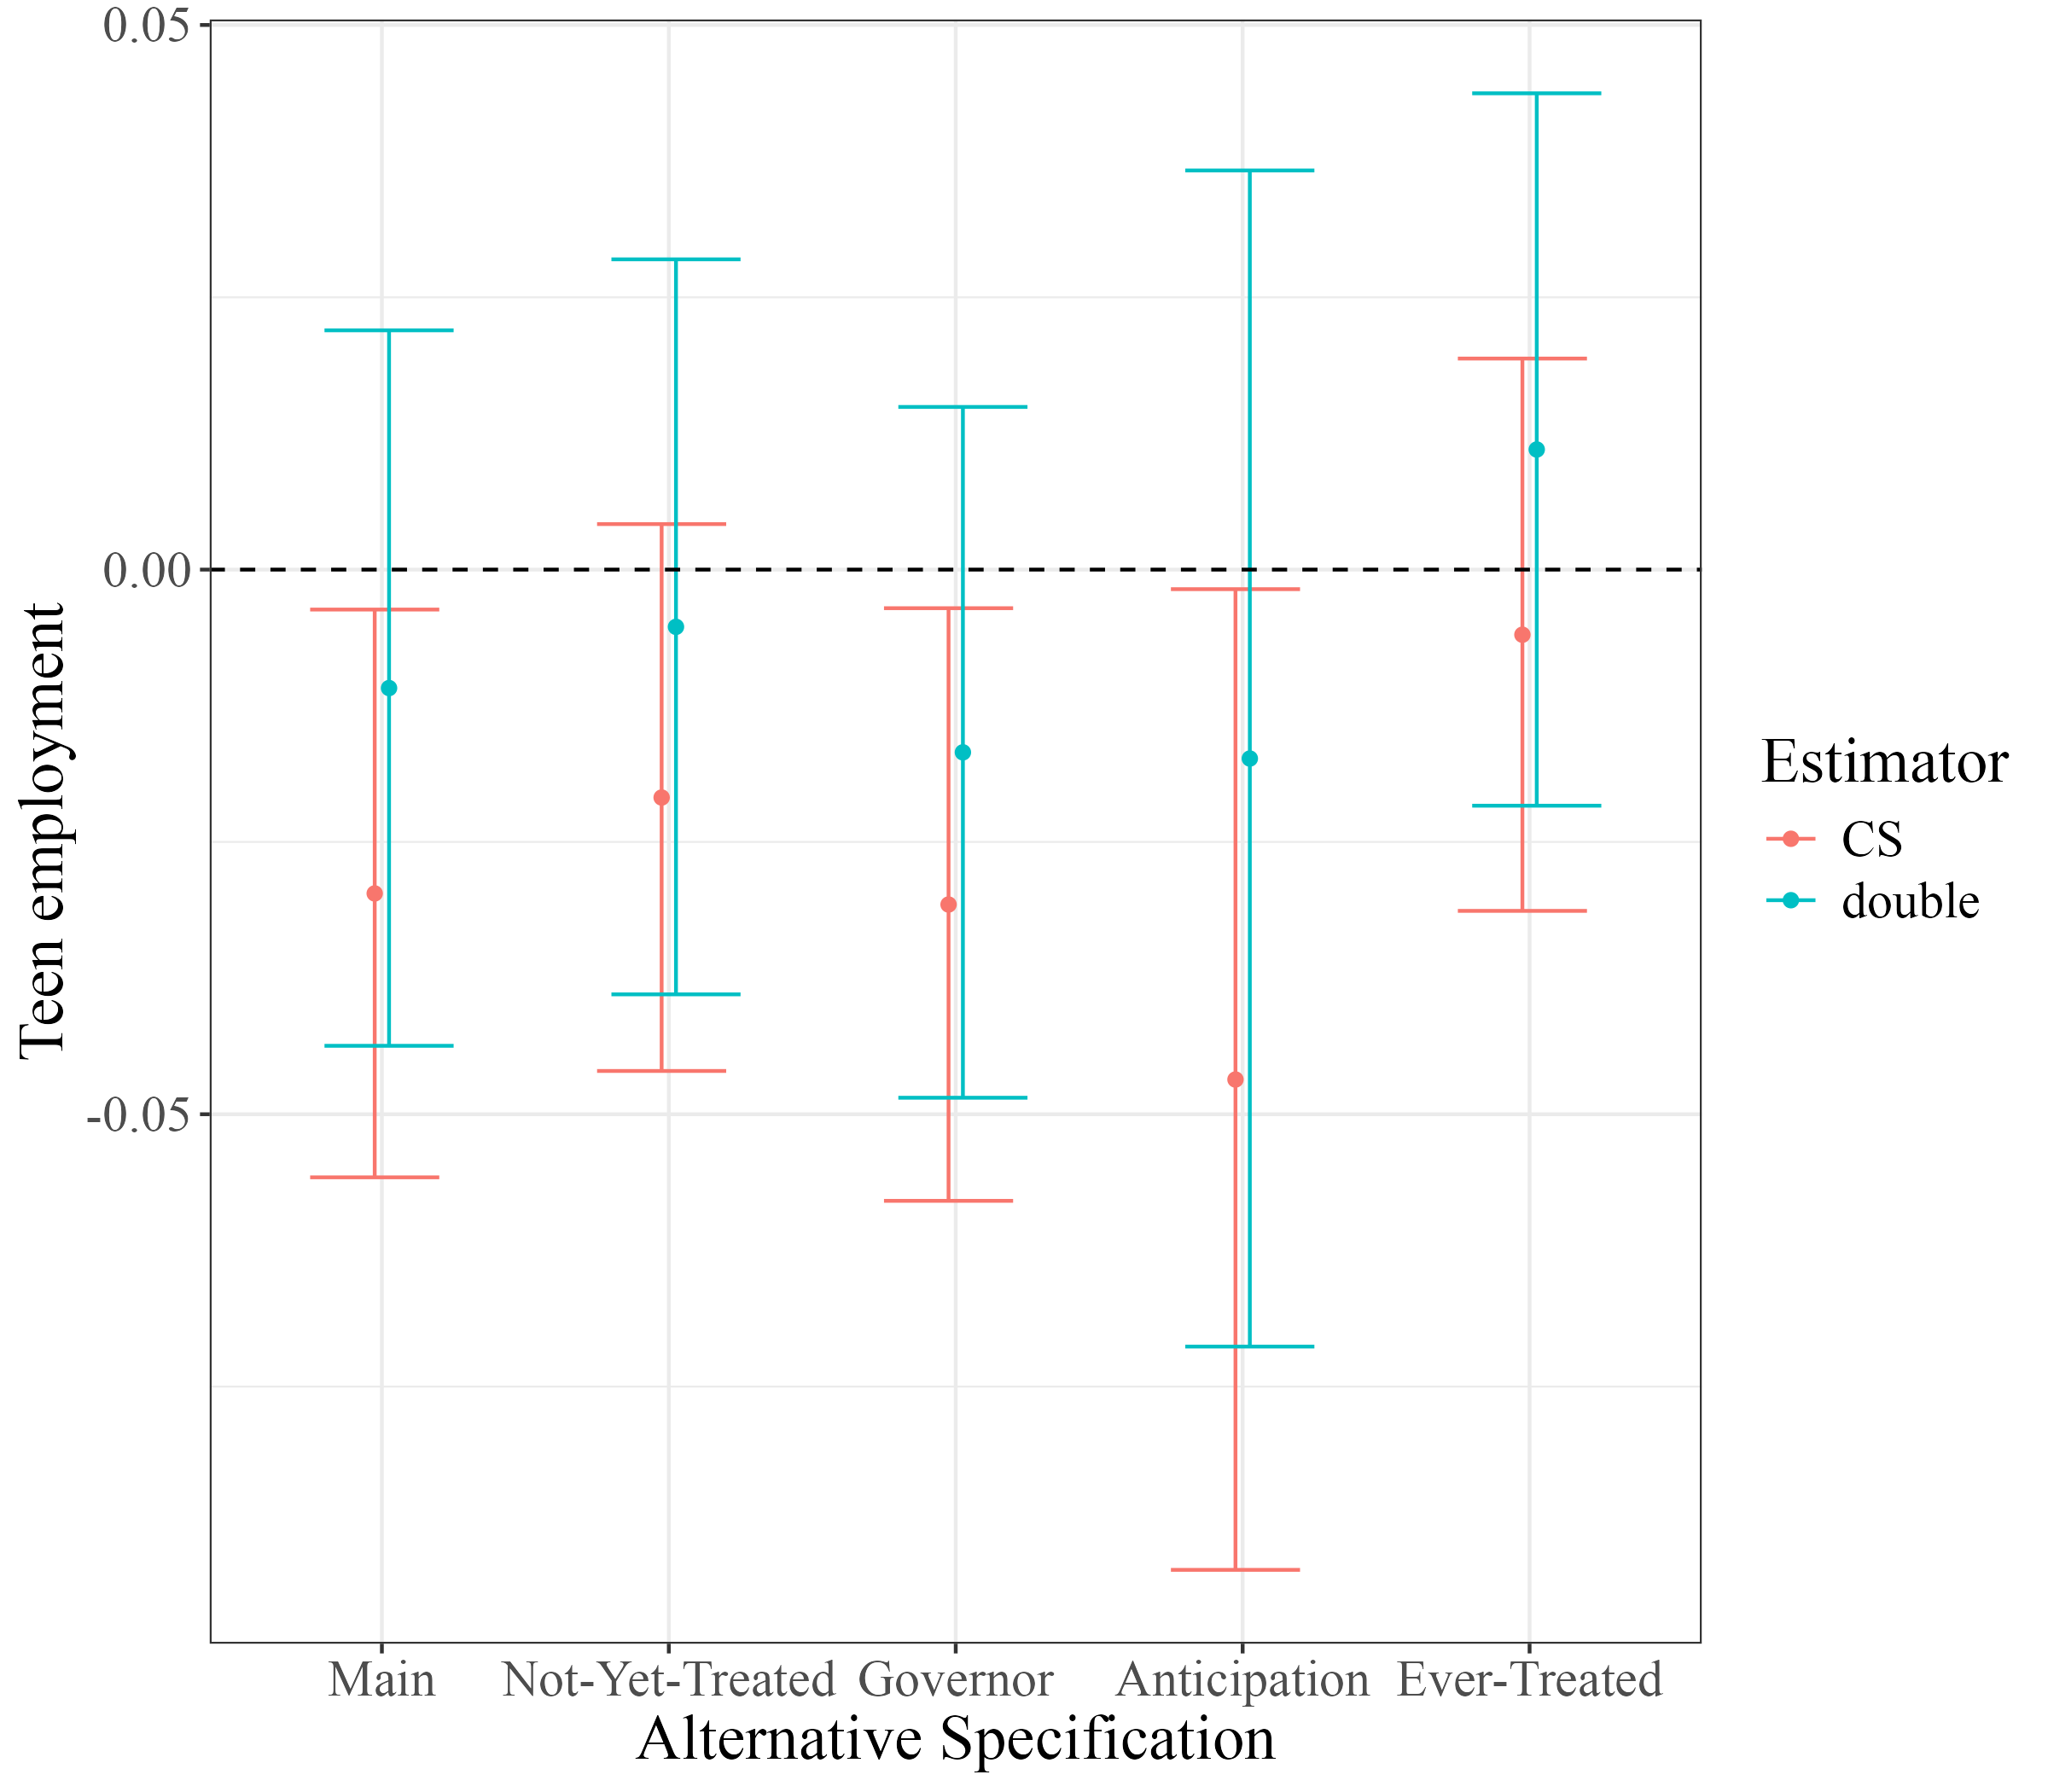} 
    \label{fig:rob}
\end{figure}

\end{frame}
